# Supplementary material for: PanelPRO: A R package for multi-syndrome, multi-gene risk modeling for individuals with a family history of cancer
Source: arXiv:2010.13011 source file (2020-10-25)
Supplement: Supplementary file 1 [file appendix.tex]

\appendix

\section{Appendices}
\label{sec:appendix}

\subsection{Cancer name mapping}
\label{subsec:cancer_names}

\begin{table}[H]
	\centering
\begin{tabular}{ll}
	\toprule
	Short name & Long name \\ 
	\midrule 
	BRA & Brain \\
	BC & Breast \\
	CER & Cervical \\
	COL & Colorectal \\
	ENDO & Endometrial \\
	GAS & Gastric \\
	KID & Kidney \\
	LEUK & Leukemia \\
	MELA & Melanoma \\
	OC & Ovarian \\
	OST & Osteosarcoma \\
	PANC & Pancreas \\
	PROS & Prostate \\
	SMA & Small intestine \\
	STS & Soft Tissue Sarcoma\\
	THY & Thyroid \\
	UB & Urinary Bladder\\
	HEP & Hepatobiliary \\
% 	CBC & Contralateral breast\\
	\bottomrule
\end{tabular}
	\caption{Abbreviations of cancers in \textbf{PanelPRO}.}
	\label{tab:cancer_mapping}
\end{table}
